# Supplementary material for: AdaAfford: Learning to Adapt Manipulation Affordance for 3D Articulated Objects via Few-shot Interactions
Source: arXiv:2112.00246 source file (2023-05-04)
Supplement: Supplementary file 2 [file supp_failure.tex]

\section{Failure Cases and Analysis}

\begin{figure}[t]
    \begin{center}
        \includegraphics[width=\linewidth, 
        trim={0cm, 0cm, 0cm, 0cm}, clip]{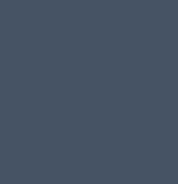}
    \end{center}
    \caption{\textbf{Failure Cases.}
    }
    \label{fig:failure}
\end{figure}
